# Supplementary material for: Larth: Dataset and Machine Translation for Etruscan
Source: arXiv:2310.05688 source file (2023-10-09)
Supplement: Supplementary file 1 [file appendix.tex]

\appendix\label{sec:appendix}
\section{Etruscan examples}
\begin{table}[H]
    \centering
    \begin{tabular}{l|l}
        \multicolumn{2}{c}{\textbf{ETP}}  \\
        % \hline
        ETT: & cleusinas : laris : larisal : clan \\
        ENG: & Laris Cleusinas, son of Laris.\\
        \hline
        ETT: &  mi karkanas {\texttheta}ahvna \\
        ENG: &  I (am) the container of Karkana \\
        \hline
        ETT: &  mi e.i. mi.n.pi capi mi numar | \\
        & {\texttheta}evru.c.l.na.s. | qupe.s. fulu.{\'\textvarsigma}.la \\
        ENG: &  Don't take me. I (am) nunar.\\
        & (I am the property) of Qupe\\
        & Thevrudnas, the (son) of Fulu. 
        \\ 
    \end{tabular}
    \caption{Examples from ETP portion of the dataset. Etruscan text is not transcribed.}
    \label{tab:example_etp}
\end{table}

\begin{table}[H]
    \centering
    \begin{tabular}{l|l}
        \multicolumn{2}{c}{\textbf{CIEP}}  \\
        ETT: & a--l----- \\
        ENG: & mr-auleslave\\
        \hline
        ETT: &  visl  \\
        ENG: &  of-the-goddess-vipsi \\
        \hline
        ETT: & tularspu \\
        ENG: &  boundaries\\
    \end{tabular}
    \caption{Examples from CIEP portion of the dataset. The texts are not normalised and they are often noisy.}
    \label{tab:example_ciep}
\end{table}

\section{Grammatical features}
% \note{List grammatical features}
% \bottomcaption{some caption}
\begin{supertabular}{l}
    % \centering
    % \begin{tabularx}{l}
        \textbf{List of grammatical features} \\
        city name \\
        place name \\
        name \\
        epithet \\
        theonomin \\
        cognomen \\
        praenomen \\
        nomen \\
        nominative \\
        accusative \\
        masculine \\
        feminine \\
        nas-particle \\
        nasa-particle \\
        u-particle \\
        θ-imperative \\
        θ-particle \\
        θas-particle \\
        as-particle \\
        active \\
        passive \\
        non-past \\
        past \\
        imperative \\
        jussive \\
        necessitative \\
        inanimate \\
        animate \\
        indefinite (pronoun) \\
        definite (article) \\
        deictic particle \\
        enclitic particle \\
        enclitic conjunction \\
        demonstrative \\
        adverb \\
        article \\
        conjunction \\
        post-position \\
        pronoun \\
        relative \\
        subordinator \\
        negation \\
        numeral \\
        1st genitive \\
        2nd genitive \\
        1st ablative \\
        2nd ablative \\
        locative \\
        1st pertinentive \\
        2nd pertinentive \\
        1st person \\
        2nd person \\
        3rd person \\
        plural\\
    \noalign{\captionof{table}{List of grammatical features describing the words in the Etruscan dictionary}}\\
    \label{tab:features}\\
\end{supertabular}

\section{Translation examples}
\note{Show random examples from the models}
\subsection{Random model}
\begin{table}[H]
\begin{tabular}{ll}
    \multicolumn{2}{l}{\textbf{ETP+CIEP}}\\
    Etruscan: & lethial \\
    Reference: & s lethis \\
    Prediction: & o and wife thegoddessminerva \\
    & ancestorsthree s munis
\end{tabular}
\end{table}

\begin{table}[H]
\begin{tabular}{ll}
    \multicolumn{2}{l}{\textbf{ETP}}\\
    Etruscan: & eca : σ'uθic : velus : ezpus | \\
     & clensi : cerine \\
    Reference: & this funerary monument belongs\\
    & to vel etspu it is constructed \\
    & by his son \\
    Prediction: & from wife and sani the of victim \\
    & ceisui \\
\end{tabular}
\end{table}

\subsection{Dictionary model}

\begin{table}[H]
\begin{tabular}{ll}
    \multicolumn{2}{l}{\textbf{White space tokenizer}} \\
    Etruscan: & itun turuce venel atelinas tinas \\
    & dlniiaras \\
    Reference: & venel atelinas dedicated this vase \\
    & to the sons of tinia \\
    Prediction: & this dedicated venel atelina tinia \\
\end{tabular}
\end{table}
\begin{table}[H]
\begin{tabular}{ll}
    \multicolumn{2}{l}{\textbf{Suffix tokenizer}} \\
     Etruscan: & itun turuce venel atelinas tinas\\
     & dlniiaras\\
    Reference: & venel atelinas dedicated this vase\\
    & to the sons of tinia\\
    Prediction: & this for him dedicated three this \\
    & venel laris atelina   shows  \\
\end{tabular}
\end{table}
\subsection{N-grams and Na\"ive Bayes model}

\begin{table}[H]
\begin{tabular}{ll}
    \multicolumn{2}{l}{\textbf{Ett, no order}} \\
    Etruscan: & eca shuthic velus ezpus clensi \\
    & cerine \\
    Reference: & this funerary monument belongs \\
    & to vel etspu it is constructed\\
    & by his son\\
    1-grams: & an of velethnai of tablet of \\
    2-grams: & cavatha \\
    3-grams: & of \\
\end{tabular}
\end{table}

\begin{table}[H]
\begin{tabular}{ll}
    \multicolumn{2}{l}{\textbf{Ett, order}} \\
    Etruscan: & eca shuthic velus ezpus clensi \\
    & cerine \\
    Reference: & this funerary monument belongs \\
    & to vel etspu it is constructed\\
    & by his son\\
    1-grams: & an of velethnai of tablet of \\
    2-grams: & cavatha \\
    3-grams: & of \\
\end{tabular}
\end{table}

\begin{table}[H]
\begin{tabular}{ll}
    \multicolumn{2}{l}{\textbf{Ett-Eng, no order}} \\
    Etruscan: & eca shuthic velus ezpus clensi \\
    & cerine \\
    Reference: & this funerary monument belongs \\
    & to vel etspu it is constructed\\
    & by his son\\
    1-grams: & of of of of of of\\
    2-grams: & \\
    3-grams: & \\
\end{tabular}
\end{table}

\begin{table}[H]
\begin{tabular}{ll}
    \multicolumn{2}{l}{\textbf{Ett-Eng, order}} \\
    Etruscan: & eca shuthic velus ezpus clensi \\
    & cerine \\
    Reference: & this funerary monument belongs \\
    & to vel etspu it is constructed\\
    & by his son\\
    1-grams: & of the was of of of\\
    2-grams: & \\
    3-grams: & \\
\end{tabular}
\end{table}

\begin{table}[H]
\begin{tabular}{ll}
    \multicolumn{2}{l}{\textbf{Na\"ive Bayes models }} \\
    Etruscan: & eca shuthic velus ezpus \\
     & clensi cerine \\
    Reference: & this funerary monument \\
    & belongs to vel etspu it is \\
    & constructed by his son \\
    Ett., bigrams: & cavatha cavatha citadel \\
    & citadel saturnies \\
    & saturnies paithinas \\
    Ett, trigrams: & of still cavis palpe palpe \\
    & saturnies eight eight \\
    Ett-Eng, bigrams: & saturnies saturnies \\
    & saturnies saturnies \\
    & parx x \\
    Ett-Eng, trigrams: & saturnies cushu saturnies \\
    & saturnies saturnies \\
    & saturnies saturnies \\
\end{tabular}
\end{table}

\subsection{IBM models}
\begin{table}[H]
\begin{tabular}{ll}
    \multicolumn{2}{l}{\textbf{ETP}} \\
    Etruscan: & eca shuthic velus ezpus \\
    & clensi cerine \\
    Reference: & this funerary monument belongs\\
    & to vel etspu it is constructed by \\
    & his son\\
    IBM1: & ersce funerary rapi etspus erected\\
    & is\\
    IBM2: & this funerary vel etspus son \\
    & constructed\\
    IBM3: & this funerary vel etspus son \\
    & constructed\\
    IBM4: & this funerary vel etspus son \\
    & constructed\\
    IBM5: & this funerary vel etspus son \\
    & constructed\\
\end{tabular}
\end{table}

\begin{table}[H]
\begin{tabular}{ll}
    \multicolumn{2}{l}{\textbf{ETP+CIEP}} \\
    Etruscan: & lethial \\
    Reference: & s lethis\\
    IBM1: & lethis\\
    IBM2: & lethis\\
    IBM3: & \\
    IBM4: & \\
    IBM5: & \\
\end{tabular}
\end{table}

\subsection{Transformer Models - Larth}
% ETP
    % Repeat
    % Spce
    % char
    % word
    % Lat
    % Grc
    
% ETP+CIEP
    % Repeat
    % Spce
    % unk
    % name
    % char
    % word
    % Lat
    % Grc

\section{Larth hyperparameters}
\begin{table}[H]
    \centering
    \begin{tabular}{l l}
        \multicolumn{2}{l}{\textbf{Larth hyperparameters and settings}}\\
        activation\_fn & gelu \\
        attention\_dropout & 0.1 \\
        block\_size & 8 \\
        char\_vocab\_size & \textit{from tokenizer} \\
        decode & \textit{from train/test} \\
        deterministic & \textit{from train/test} \\
        dropout & 0.1 \\
        dtype & float32 \\
        emb\_size & 256 \\
        encoder\_type & \textit{from experiment} \\
        layers & 1 \\
        max\_len & 256 \\
        mlp\_dim & 512 \\
        num\_heads & 8 \\
        num\_rand\_blocks & 3 \\
        out\_char\_vocab\_size& \textit{from tokenizer} \\
        out\_word\_vocab\_size& \textit{from tokenizer} \\
        qkv\_dim & 256 \\
        word\_char\_emb\_size & 256 \\
        word\_vocab\_size & \textit{from tokenizer} \\
    \end{tabular}
    \caption{Settings and hyperparameters used to run Larth. Some values depend on the tokenizer, while others depend on whether we are training the model or testing it.}
    \label{tab:larth-setting}
\end{table}

\begin{table}[H]
    \centering
    \begin{tabular}{l l}
        \multicolumn{2}{l}{\textbf{Training configuration}}\\
        batch\_size & 32 \\
        beam\_size & 1 \\
        cached & true \\
        checkpoint\_every\_epochs & 50 \\
        data\_path & \textit{from experiment} \\
        dataset\_type & \textit{from experiment} \\
        debug & false \\
        epochs & 1000 \\
        etruscan\_vocab & EPT\_POS.csv \\
        eval & true \\
        eval\_every\_epochs & 50 \\
        label\_smoothing & 0.1 \\
        length\_penalty & 0.6 \\
        lr & 0.002 \\        
        name\_augmentation- & \multirow{2}*{\textit{from experiment}} \\
        -\_max\_replacements & \\
        restore\_checkpoints & false \\
        restore\_from & null \\
        seed & 0 \\
        source\_lang & etruscan \\
        source\_model & all\_small \\
        subset & \textit{from experiment} \\
        target\_lang & english \\
        target\_model & all\_small \\
        train & true \\
        train\_size & 0.9 \\
        unk\_augmentation\_iterations & 0 \\
        unk\_augmentation\_len & 1.0 \\
        unk\_augmentation\_prob & 0.0 \\
        warmup\_steps & 250 \\
        weight\_decay & 0.0001 \\
        workdir & \textit{from experiment} \\
    \end{tabular}
    \caption{Training configuration for Larth.}
    \label{tab:train_settings}
\end{table}
